# Supplementary material for: AI-CARGO: A Data-Driven Air-Cargo Revenue Management System
Source: arXiv:1905.09130 source file (2019-05-22)
Supplement: Supplementary file 1 [file appendices.tex]

\section{Appendix: Terminology}
\begin{table}[h]
\begin{tabular}{|l|l|} \hline
Term & Description  \\ \hline \hline
bkdvol & the intial booked volume \\ \hline
rcsvol & the final received volume \\ \hline

\end{tabular}
\end{table}
\section{Appendix: Log-Normal Distribution}
Suppose we want to generate samples from a log-normal distribution with mean $\mu$ and standard deviation $\sigma$. Then
before we can invoke a standard function $rlnorm(a,b)$, we need to transform the mean and standard deviation to $a$ and
$b$ which are the location and shape parameters.
